# Supplementary material for: RED-Attack: Resource Efficient Decision based Attack for Machine Learning
Source: arXiv:1901.10258 source file (2019-01-30)
Supplement: Supplementary file 1 [file Appendix.tex]

\section{Mathematical Formulation of RED-Attack}\label{formulations}
To formulate our attack, we use the commonly used cost function defined by the CW attack.
\[cost = c \times (f(X_{adv}) - f(X_{target}))^2 +  \sum{(X - X_{adv})^2}\]

Note that our main goal behind defining the above cost function is to minimize \((f(X_{adv}) - f(target))^2\) and \(\sum{(\Delta_x)^2}\) simultaneously. However, the problem with this cost function is that, in our case, \(f\) is discrete and hence its gradients \textcolor{red}{can we write that the function is not differentiable?} are not available to perform the optimization. Therefore, we reformulate the above cost as,

\[cost = c \times (f(X_{adv}) != f(X_{target})) + \sum{(X - X_{adv})^2}\]

Note that if \(c\) is very large, the value of the cost function will be very large when \(X_{adv}\) belongs to some class other than the target class, and the gradient of the cost can be approximated as

\[\frac{\partial cost}{\partial X_{adv}} = X_{adv} - X_{target}\]

Similarly, if the current adversarial image is an instance of the target class, the gradient can be approximated as

\[\frac{\partial cost}{\partial X_{adv}} = 2 \times (X_{adv} - X)\]

And the new adversarial instance is computes as,

\[X_{adv,new} = X_{adv,old} - \alpha \times \frac{\partial cost}{\partial X_{adv}}\]

We note two main points here. First, the two gradients computed only allow us to move in linear fashion, either towards the target example or towards the source example until we reach the boundary. We accomplish this more efficiently by using binary stepping as shown in Algorithm \ref{TBE} and Algorithm \ref{UBE}. Secondly, mere linear updates either towards the target example or towards the source example, will cause infinite oscillations at the transition of the boundary. To counter this problem, we redefine our cost function for the region characterized by the \(\delta_{min}\) distance of each pixel to the boundary. The new cost function is,
\[cost = \sum{(X_{adv} - X)^2}\]

We optimize this new cost function using stochastic Zeroth-Order Optimization. First we randomly select \(n\) number of pixels in the \(X_{adv}\) and introduce random perturbations in the selected pixels to compute \(\overset{-}{X}_{adv}\). The zeroth-order gradient is,

\[\frac{\partial cost}{\partial X_{adv}} = \frac{\sum{(X_{adv} - X)^2} - \sum{(\overset{-}{X}_{adv} - X)^2}} {X_{adv} - \overset{-}{X}_{adv}}\]

\[X_{adv,new} = X_{adv,old} - \lambda \times \frac{\partial cost}{\partial X_{adv}}\]

The magnitude of ``\(\lambda\)'' is adjusted efficiently to make a jump that brings the adversarial examples closest to the source example.

\section{Generating Adversarial Examples}\label{Targted_Attacks}

\begin{figure}[t!]
	\centering
	\includegraphics[width=1\linewidth]{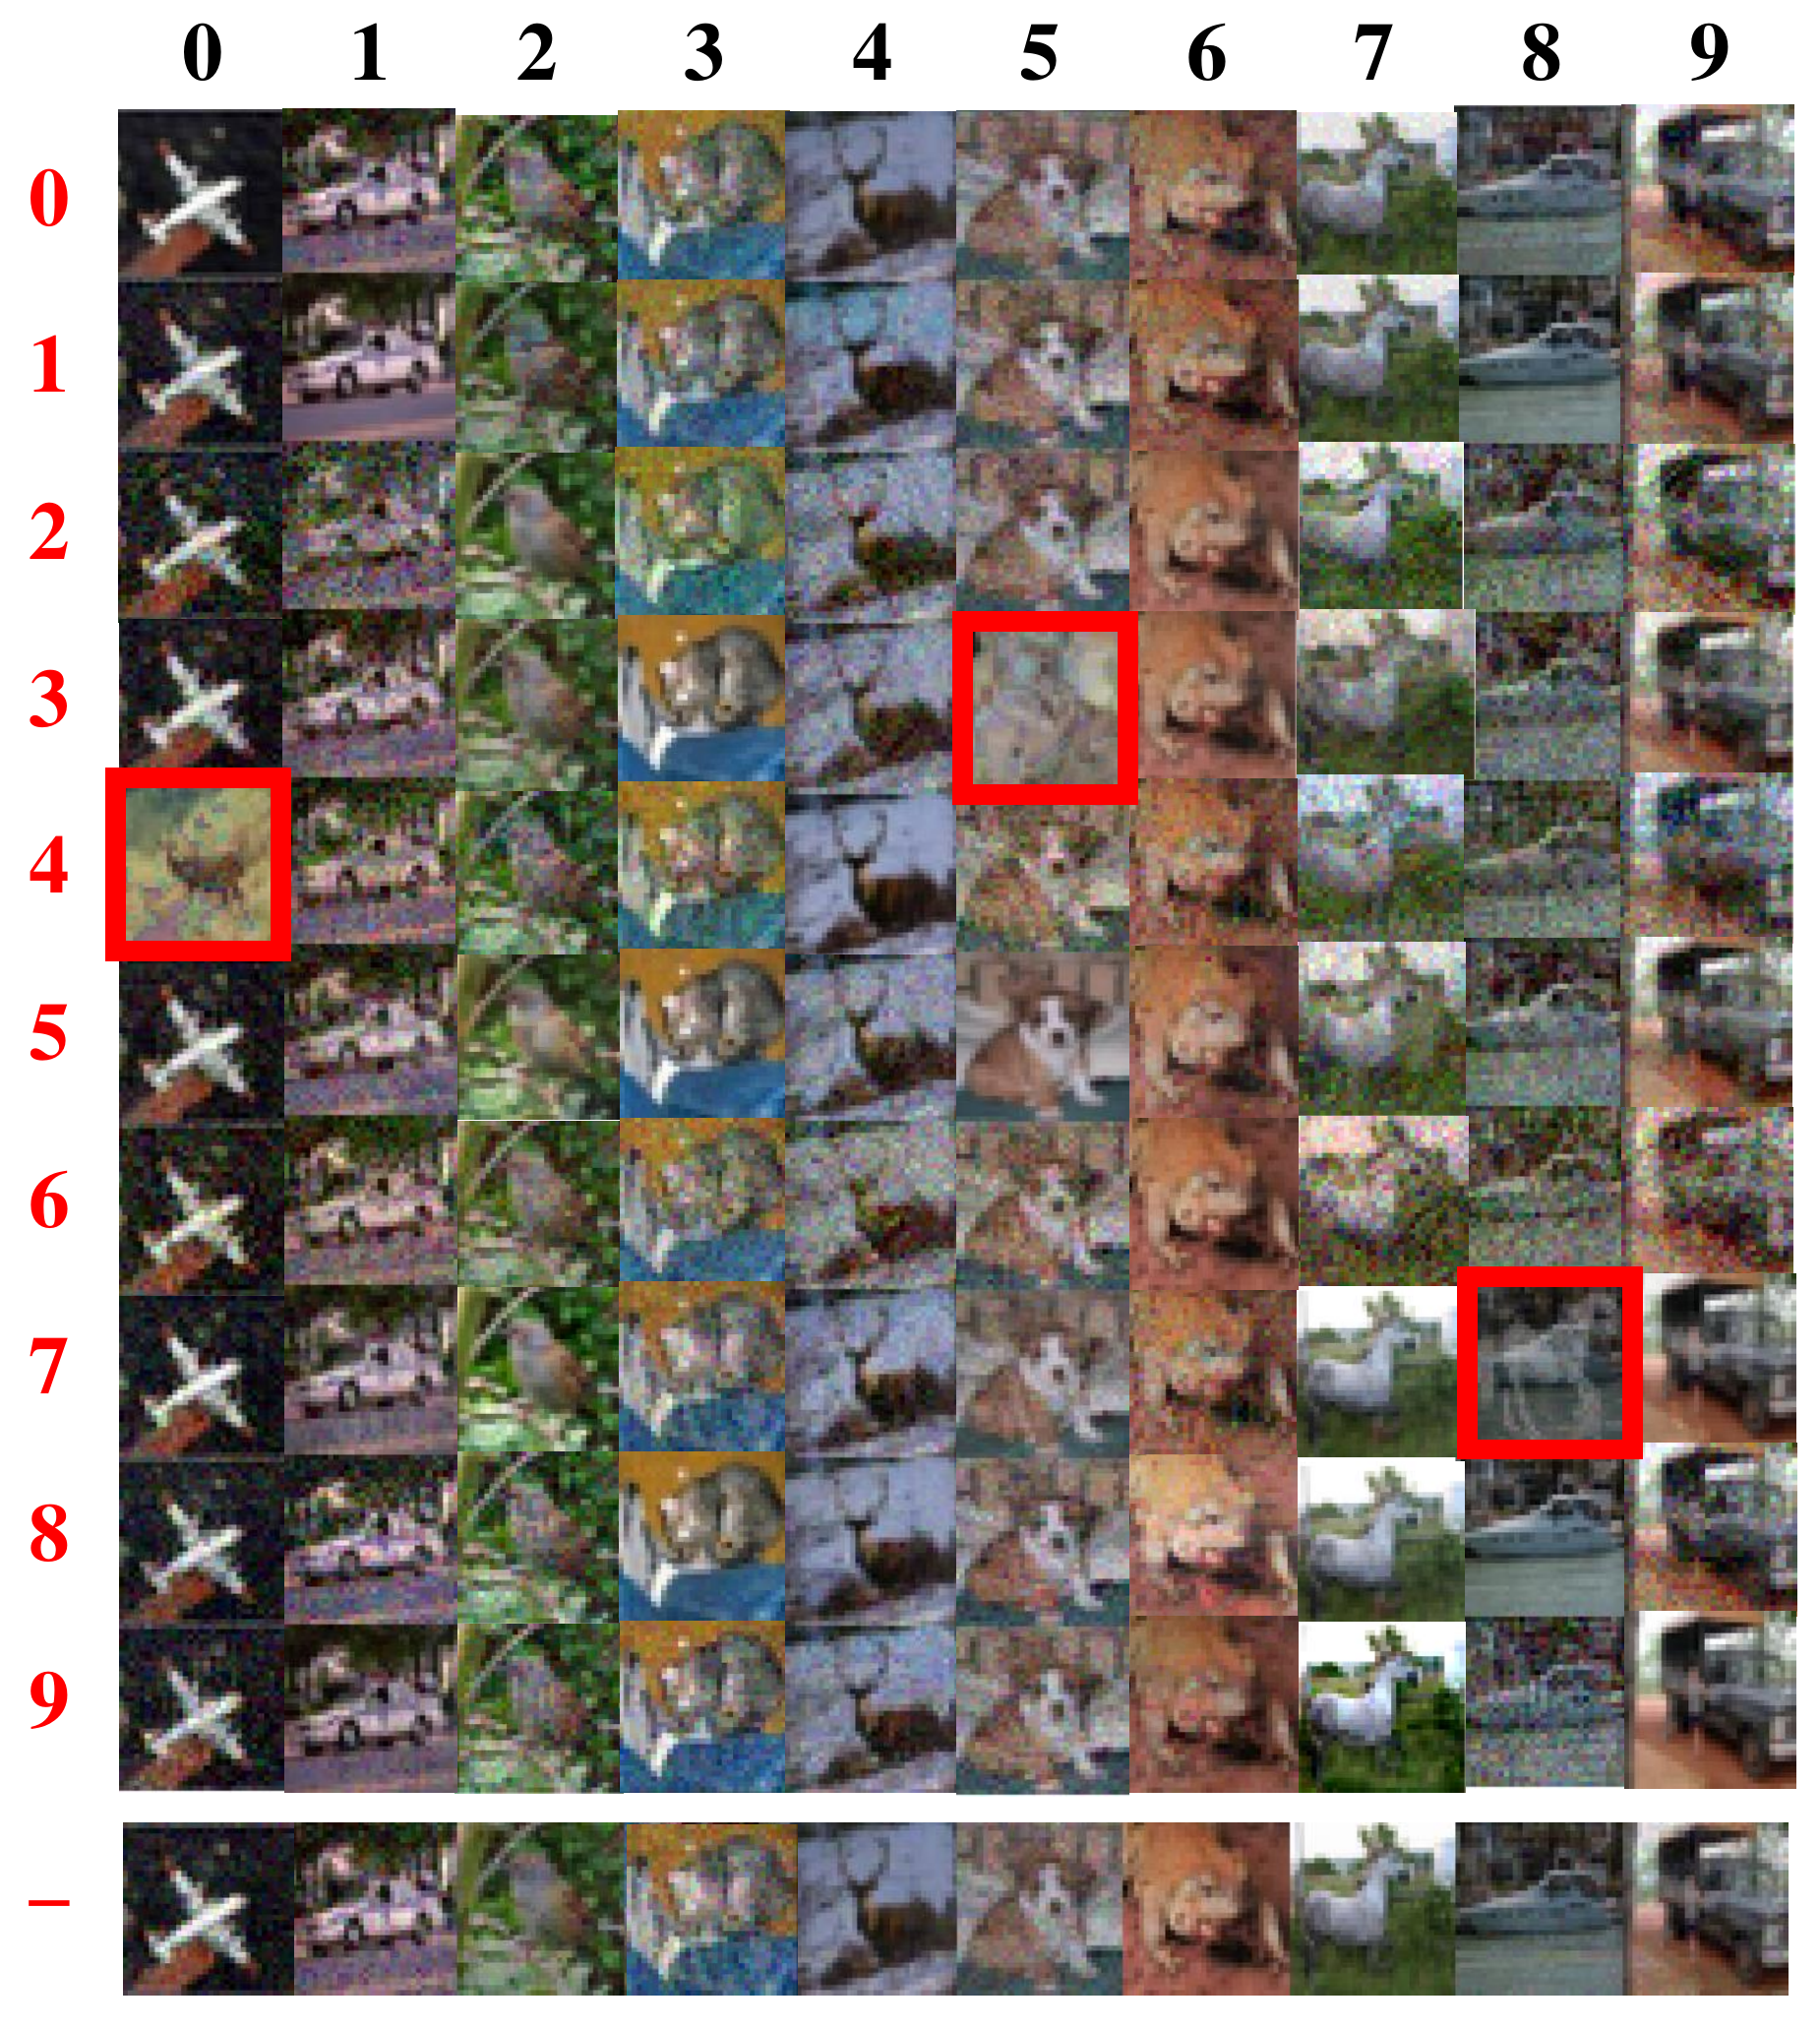}
	
	\caption{\textit{Performing the Targeted and Un-targeted Attacks on the classifier using only the decision provided by the classifier. (Top 10 rows) Adversarial examples found for the targeted attacks. Correct labels are shown top in black on top. The target labels are shown in red on left. (Last Row) Adversarial examples found for un-targeted attacks. Maximum number of queries = \(10^5\)}}
	\label{fig:AiO}
\end{figure}

Adversarial examples found for the targeted and un-targeted attack scenarios against the black-box classifier are reported in Figure \ref{fig:AiO}.

Three images have been highlighted. We find that these images are similar to the images used as initial targets for them. In other words, our black-box attack fails to find a satisfactory adversarial example in these cases. However, we repeat the experiment for the same source and target image several times and find that the algorithm never fails again. There may be many reasons as to why it failed for the first time. The simplest one being a rare encounter of the local minima or the saddle point.

\section{Targeted Trends}\label{Targted_Attacks}

\begin{figure*}[t!]
	\centering
	\includegraphics[width=1\linewidth]{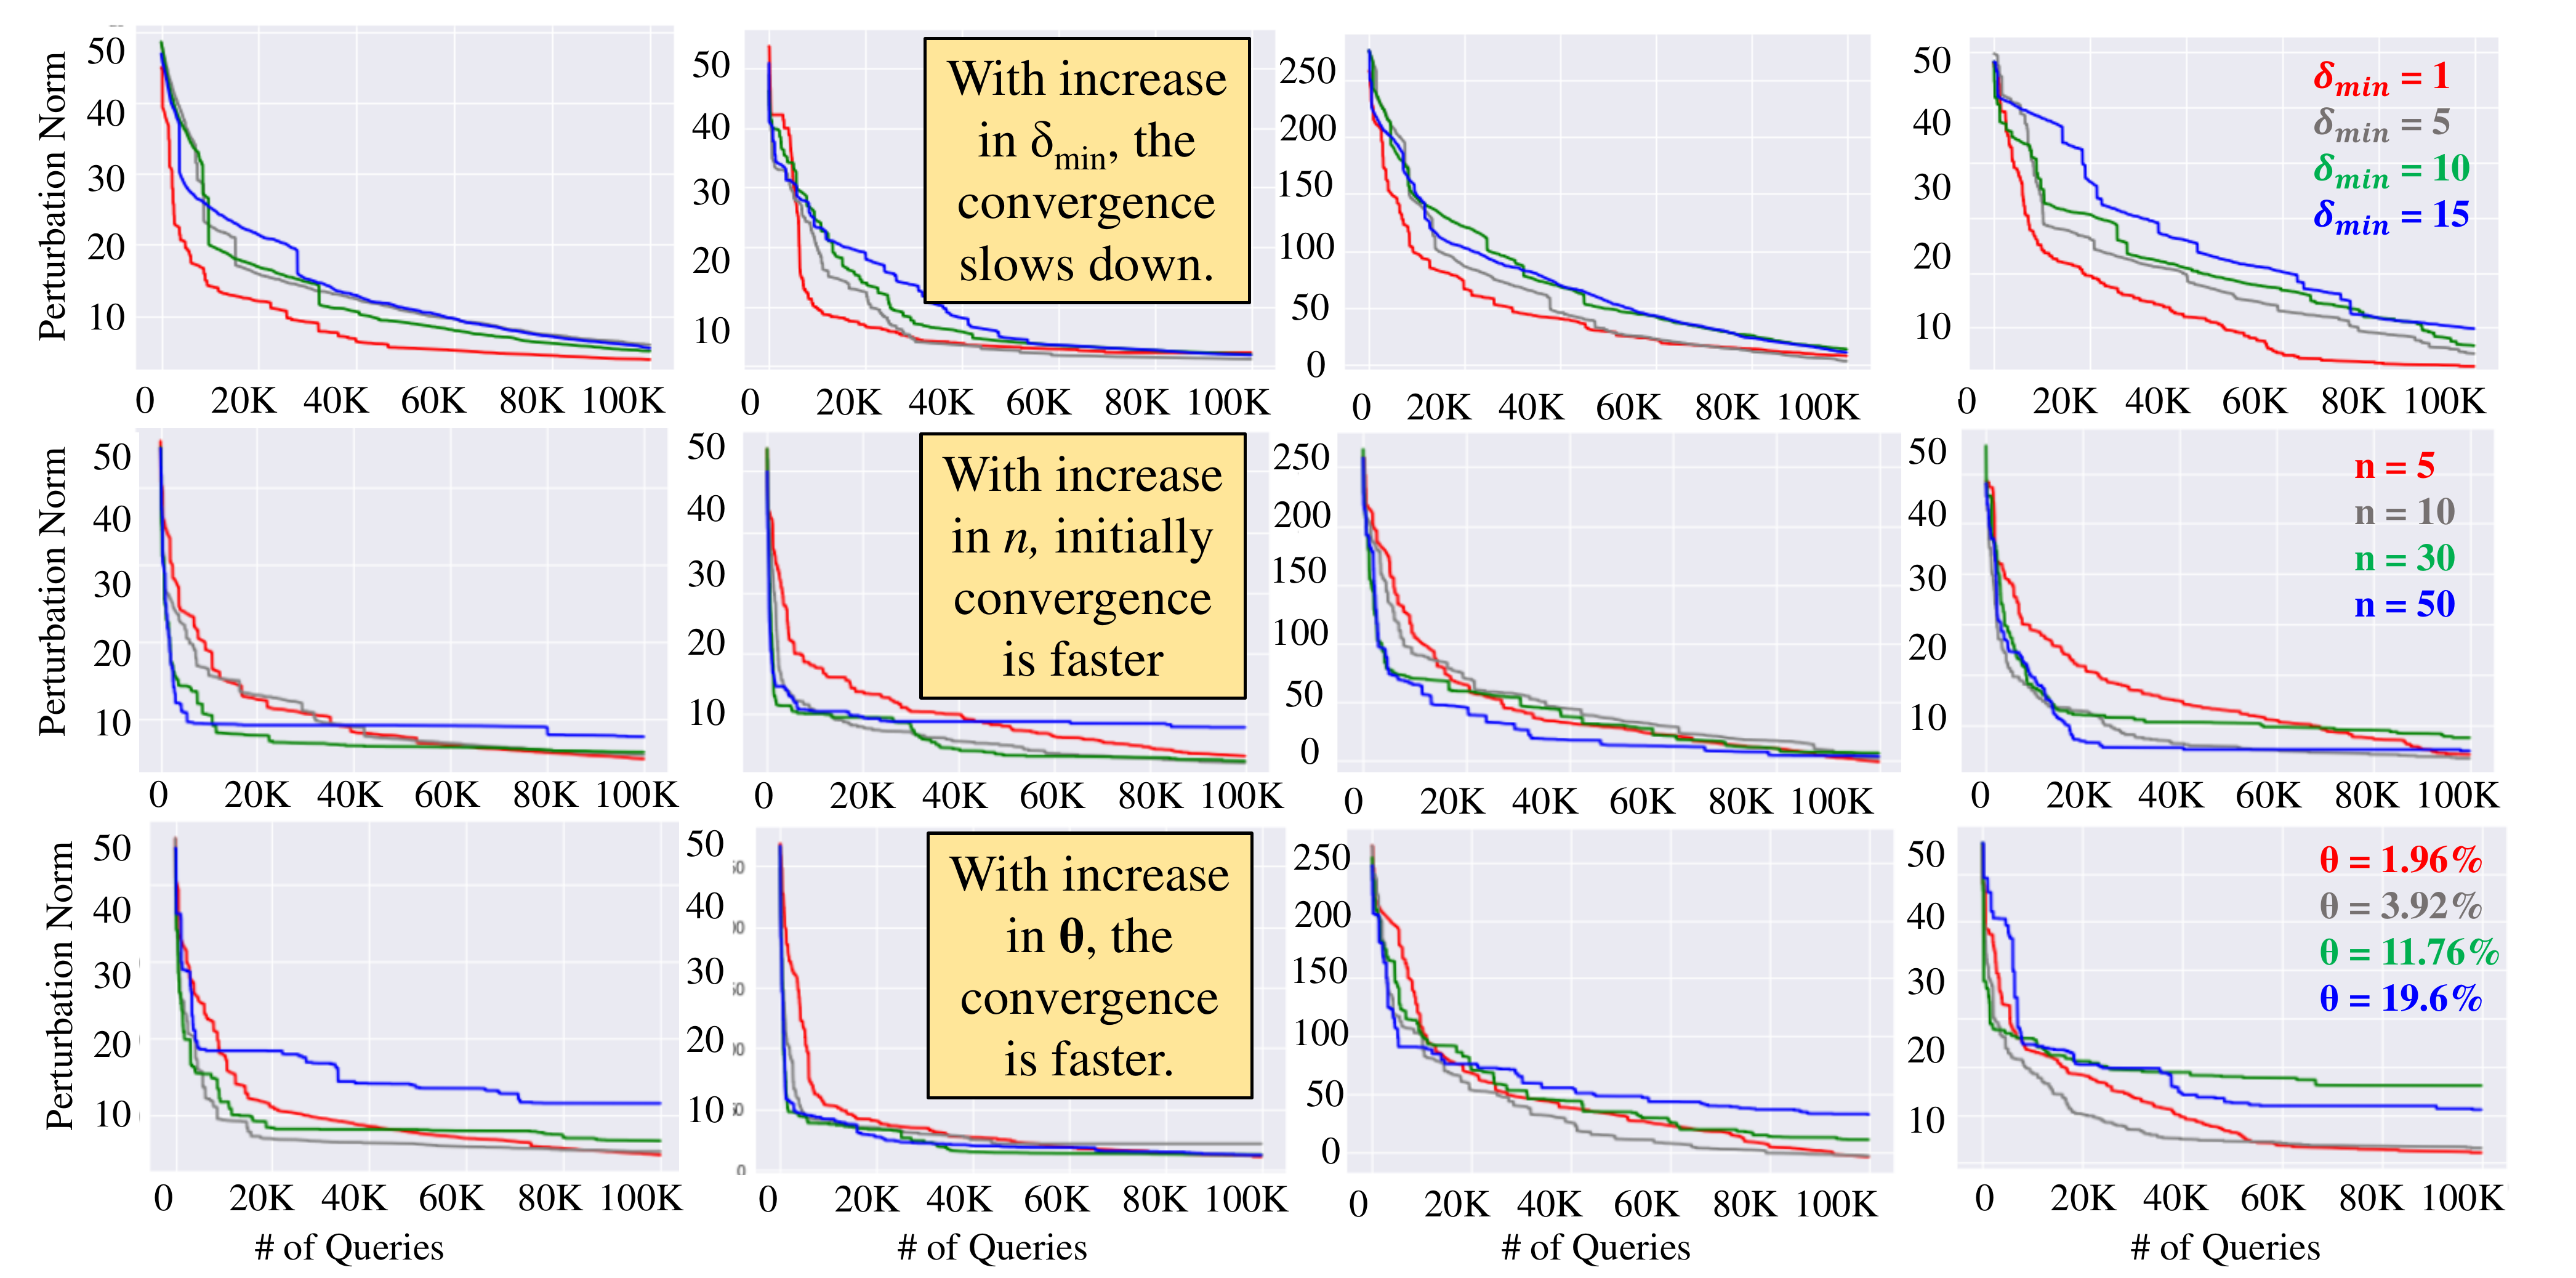}
	\caption{\textit{The trends of distance (d) of the adversarial example from the corresponding source examples as the algorithm progresses, for various values of \(\theta\). \(\delta_{min} and n\). (From left to right) Truck classified as airplane, truck classified as a car, truck classified as a bird, truck classified as a cat}}
	\label{fig:P_Plot_T}
\end{figure*}
